# Supplementary material for: Foundational Large Language Models for Materials Research
Source: arXiv:2412.09560 source file (2025-01-28)
Supplement: Supplementary file 1 [file appendix_a.tex]

\section{Pre-training and fine-tuning datasets}

\begin{table}[H]
\centering
\label{tab:data_pre_fine}
\scalebox{0.9}{
    \begin{tabular}{ccc}
    \toprule
    \textbf{Pretraining} &   &   \\ \midrule
    \textbf{Source} & \textbf{Size} &  \textbf{Description} \\ \midrule
    Research papers & 4 Millions & 396/598 \\ 
    comptable & 0.812 & 0.834 \\ 
    regextable & 0.879 & 0.848 \\ 
    glass id & 0.804 & 0.734 \\
    composition labels & 0.677 & 0.28 \\
    chemical labels & 0.673 & 0.582 \\ 
    \bottomrule
    \end{tabular}
    }
    \caption{results on DiSCoMaT}
\end{table}
